# Supplementary material for: Thresholding Bandits with Augmented UCB
Source: arXiv:1704.02281 source file (2019-06-07)
Supplement: Supplementary file 1 [file appendix.tex]

\appendix

\section{Cumulative Regret Bound}

\begin{theorem}
\label{proofTheorem:Prop:1}
The regret $R_T$ for AugUCB satisfies
\begin{align*}
&\E [R_{T}]\\
& \leq \sum\limits_{i\in A:\Delta_{i} > b}\bigg\lbrace \dfrac{T\Delta_{i}}{( \frac{3}{2} T\Delta_i^{2})^{\psi_{m_i}}}
  + \left( \Delta_i +\dfrac{22\Delta_i\psi_{m_i}\log( \frac{3}{2} T\Delta_i^2)}{ \Delta_i}\right)\\
  & \bigg(\dfrac{4T^{1-\psi_{m_i}}2^{\psi_{m_i}-\frac{1}{2}}}{\Delta_{i}^{\psi_{m_i}-\frac{1}{2}}} \bigg)\bigg \rbrace +\sum_{i\in A: 0 < \Delta_{i} \leq b}\bigg(\dfrac{4T^{1-\psi_{m_i}}2^{\psi_{m_i}-\frac{1}{2}}}{b^{\psi_{m_i}-\frac{1}{2}}} \bigg) \\
  & + \max_{\substack{i\in A: \\ \Delta_{i}\leq b}}\Delta_{i}T, \text{  for all $b\geq\sqrt{\frac{e}{T}}$}. 
\end{align*} 
\end{theorem}

\begin{proof}
\textbf{\textit{Case a: A sub-optimal arm i is not eliminated on or before round $m_{i}$ with $ * \in B_{m_i}$}}
\newline
%%%%%%%%%%%%%
For any arm $i\in A$, if it is eliminated from active set $B_{m_{i}}$ then the below two events have to come true,
\begin{align}
\hat{r}_{i} + s_{i} < \tau - s_{i}, \label{eq:armelim-var-casea1}\\
\hat{r}_{i} - s_{i} > \tau + s_{i}, \label{eq:armelim-var-caseb1}
\end{align}

From Theorem \ref{Result:Theorem:1}, we know that a sub-optimal arm $i\in\mathcal{A}$, the probability that it is not correctly eliminated in the $m_i$-th round (or before) is also bounded by $4\exp\left(- \dfrac{3\rho \psi_{m_i}}{2} \left(\dfrac{\sigma_{i}^{2}+\sqrt{\rho\epsilon_{m_{i}}}+1}{3\sigma_{i}^{2}+\sqrt{\rho \epsilon_{m_{i}}}}\right) \log( T\epsilon_{m_{i}}) \right)$.

Summing over all arms in $\mathcal{A}^{'}$ and trivially bounding the regret for each arm $i\in \mathcal{A}^{'}$,

\begin{align*}
&\sum_{i\in A^{'}}T\Delta_{i}\exp\left(- \dfrac{3\rho \psi_{m_i}}{2} \left(\dfrac{\sigma_{i}^{2}+\sqrt{\rho\epsilon_{m_{i}}}+1}{3\sigma_{i}^{2}+\sqrt{\rho \epsilon_{m_{i}}}}\right) \log( T\epsilon_{m_{i}}) \right)\\
&\overset{(a)}{\le}  \sum_{i\in A^{'}}T\Delta_{i} \exp\left(- \dfrac{3\rho \psi_{m_i}}{2} \log( T\epsilon_{m_{i}}) \right)\\
&\overset{(b)}{\le}  \sum_{i\in A^{'}}T\Delta_{i} \exp\left(-\psi_{m_i} \log( T\epsilon_{m_{i}}) \right)\\
&\overset{(c)}{\le}  \sum_{i\in A^{'}}\dfrac{T\Delta_{i}}{( T\dfrac{\Delta_i^{2}}{\rho})^{\psi_{m_i}}} \leq \sum_{i\in A^{'}}\dfrac{T\Delta_{i}}{( \frac{3}{2} T\Delta_i^{2})^{\psi_{m_i}}}
\end{align*}

In the above formulation, $(a)$ happens because  $\left(\dfrac{\sigma_{i}^{2}+\sqrt{\rho\epsilon_{m_{i}}}+1}{3\sigma_{i}^{2}+\sqrt{\rho \epsilon_{m_{i}}}}\right) \geq 1$. For $(b)$ we put $\rho=\dfrac{2}{3}$ and for $(c)$ we take the help of the inequality $\sqrt{\rho \epsilon_{m_i}} < \Delta_i$ in the $m_i$-th round.

\textbf{\textit{Case b: A sub-optimal arm i is either eliminated on or before round $m_{i}$ or there is no $ * \in B_{m_i}$}}

\textbf{\textit{Case b1: A sub-optimal arm i is in $B_{m_i}$}}

A sub-optimal arm is in $B_{m_i}$ and hence pulled no more than,
\begin{align*}
\left\lceil \dfrac{2\psi_{m_i}\log( T\epsilon_{m_i})}{\epsilon_{m_i}} \right\rceil\leq \left\lceil \dfrac{32\psi_{m_i}\log( \frac{3}{2} T\Delta_i^2)}{\frac{3}{2} \Delta_i^2}\right\rceil
\end{align*}

Hence, the total contribution to the expected regret is,
\begin{align*}
&\sum_{i\in A^{'}} \left\lceil \dfrac{32\Delta_i\psi_{m_i}\log( \frac{3}{2} T\Delta_i^2)}{\frac{3}{2} \Delta_i^2}\right\rceil\\
&\leq \sum_{i\in A^{'}} \left( \Delta_i +\dfrac{22\Delta_i\psi_{m_i}\log( \frac{3}{2} T\Delta_i^2)}{ \Delta_i}\right)
\end{align*}

\textbf{\textit{Case b2: Optimal arm ${*}$ is eliminated by a sub-optimal arm}}

	Firstly, if conditions of Case $a$ holds then the optimal arm ${*}$ will not be eliminated in round $m=m_{*}$ or it will lead to the contradiction that $r_{i}>r^{*}$. In any round $m_{*}$, if the optimal arm ${*}$ gets eliminated then for any round from $1$ to $m_{j}$ all arms ${j}$ such that $m_{j}< m_{*}$ were eliminated according to assumption in Case $a$. Let the arms surviving till $m_{*}$ round be denoted by $A^{'}$. This leaves any arm $a_{b}$ such that $m_{b}\geq m_{*}$ to still survive and eliminate arm ${*}$ in round $m_{*}$. Let such arms that survive ${*}$ belong to $A^{''}$. Also maximal regret per step after eliminating ${*}$ is the maximal $\Delta_{j}$ among the remaining arms ${j}$ with $m_{j}\geq m_{*}$.  Let $m_{b}=\min\lbrace m|\sqrt{\rho\epsilon_{m}}<\dfrac{\Delta_{b}}{2}\rbrace$. Hence, the maximal regret after eliminating the arm ${*}$ is upper bounded by, 
\begin{align*}
&\sum_{m_{*}=0}^{max_{j\in A^{'}}m_{j}}\sum_{i\in A^{''}:m_{i}>m_{*}}\bigg(\dfrac{1}{(  T\epsilon_{m_{*}})^{\psi_{m_i}}} \bigg).T\max_{j\in A^{''}:m_{j}\geq m_{*}}{\Delta}_{j}\\
&\leq\sum_{m_{*}=0}^{max_{j\in A^{'}}m_{j}}\sum_{i\in A^{''}:m_{i}>m_{*}}\bigg(\dfrac{1}{(  T\epsilon_{m_{*}})^{\psi_{m_i}}} \bigg).T.2\sqrt{\rho\epsilon_{m_{*}}}\\
&\leq\sum_{m_{*}=0}^{max_{j\in A^{'}}m_{j}}\sum_{i\in A^{''}:m_{i}>m_{*}}\bigg(\dfrac{4T^{1-\psi_{m_i}}}{\epsilon_{m_{*}}^{\psi_{m_i}-\frac{1}{2}}} \bigg)\\
&\leq\sum_{i\in A^{''}:m_{i}>m_{*}}\sum_{m_{*}=0}^{\min{\lbrace m_{i},m_{b}\rbrace}}\bigg(\dfrac{4T^{1-\psi_{m_i}}}{2^{-(\psi_{m_i}-\frac{1}{2})m_{*}}} \bigg)\\
&\leq\sum_{i\in A^{'}}\bigg(\dfrac{4T^{1-\psi_{m_i}}}{2^{-(\psi_{m_i}-\frac{1}{2})m_{*}}} \bigg)+\sum_{i\in A^{''}\setminus A^{'}}\bigg(\dfrac{4T^{1-\psi_{m_i}}}{2^{-(\psi_{m_i}-\frac{1}{2})m_{b}}} \bigg)\\
&\leq\sum_{i\in A^{'}}\bigg(\dfrac{4T^{1-\psi_{m_i}}*2^{\psi_{m_i}-\frac{1}{2}}}{\Delta_{i}^{\psi_{m_i}-\frac{1}{2}}} \bigg)+\sum_{i\in A^{''}\setminus A^{'}}\bigg(\dfrac{4T^{1-\psi_{m_i}}*2^{\psi_{m_i}-\frac{1}{2}}}{b^{\psi_{m_i}-\frac{1}{2}}} \bigg)\\
&\leq\sum_{i\in A^{'}}\bigg(\dfrac{4T^{1-\psi_{m_i}}2^{\psi_{m_i}-\frac{1}{2}}}{\Delta_{i}^{\psi_{m_i}-\frac{1}{2}}} \bigg)+\sum_{i\in A^{''}\setminus A^{'}}\bigg(\dfrac{4T^{1-\psi_{m_i}}2^{\psi_{m_i}-\frac{1}{2}}}{b^{\psi_{m_i}-\frac{1}{2}}} \bigg)\\
%& = \sum_{i\in A^{'}}\bigg(\dfrac{ C_{2}(\rho_{a}) T^{1-\rho_{a}}}{\Delta_{i}^{4\rho_{a}-1}} \bigg)+\sum_{i\in A^{''}\setminus A^{'}}\bigg(\dfrac{C_{2(\rho_{a})}T^{1-\rho_{a}}}{b^{4\rho_{a}-1}} \bigg) \text{, where } C_2(x) = \frac{2^{2x+\frac{3}{2}}x^{2x}}{\psi^{x}}
\end{align*}

%\text{, since } \sqrt{\rho_{a}\epsilon_{m}}<\dfrac{\Delta_{i}}{2}

Summing up \textbf{Case a} and \textbf{Case b}, the total expected regret is given by,
\begin{align*}
 &\sum\limits_{i\in A:\Delta_{i} > b}\bigg\lbrace \dfrac{T\Delta_{i}}{( \frac{3}{2} T\Delta_i^{2})^{\psi_{m_i}}}
  + \left( \Delta_i +\dfrac{22\Delta_i\psi_{m_i}\log( \frac{3}{2} T\Delta_i^2)}{ \Delta_i}\right)\\
  & \bigg(\dfrac{4T^{1-\psi_{m_i}}2^{\psi_{m_i}-\frac{1}{2}}}{\Delta_{i}^{\psi_{m_i}-\frac{1}{2}}} \bigg)\bigg \rbrace +\sum_{i\in A: 0 < \Delta_{i} \leq b}\bigg(\dfrac{4T^{1-\psi_{m_i}}2^{\psi_{m_i}-\frac{1}{2}}}{b^{\psi_{m_i}-\frac{1}{2}}} \bigg)
\end{align*}

% R_{T} \leq &\sum\limits_{i\in A:\Delta_{i}\geq b}\bigg\lbrace\bigg(\dfrac{2^{1+4\rho_{a}}\rho_{a}^{2\rho_{a}}T^{1-\rho_{a}}}{\psi^{\rho_{a}}\Delta_{i}^{4\rho_{a}-1}}\bigg) + \bigg(\Delta_{i}+\dfrac{32\rho_{a}\log{(\psi  T\dfrac{\Delta_{i}^{4}}{16\rho_{a}^{2}})}}{\Delta_{i}}\bigg)\\
%&  +  \bigg(\dfrac{T^{1-\rho_{a}}\rho_{a}^{2\rho_{a}}2^{2\rho_{a}+\frac{3}{2}}}{\psi^{\rho_{a}}\Delta_{i}^{4\rho_{a} -1}} \bigg) \bigg \rbrace+\sum\limits_{i\in A:0\leq\Delta_{i}\leq b}\bigg(\dfrac{T^{1-\rho_{a}}\rho_{a}^{2\rho_{a}}2^{2\rho_{a}+\frac{3}{2}}}{\psi^{\rho_{a}}b^{4\rho_{a} -1}} \bigg) + max_{i:\Delta_{i}\leq b}\Delta_{i}T

\end{proof}
